# Supplementary material for: Foliated Open Books
Source: arXiv:2002.01752 source file (2020-02-05)
Supplement: Supplementary file 1 [file appendix.tex]

% !TEX root = FOB_main.tex
%%%%%%%%%%%%%%%%%%%%%%%%%%%%%%%%%%%%%%%%%%%%%%%%%%%%%%%

\section{Appendix}
In this appendix we give a precise treatment of the neighbourhood theorem for open book foliations, and construct an explicit open book on a surface bundle to give an explicit local model for open books near surfaces with a given open book foliation. 

\begin{proposition}[Neighborhood Theorem]\label{prop:nbrh} 
Let $(B,\pi)$ and $(B',\pi')$ be open books for the 3--manifolds $M$ and $M'$ respectively. Let $\Sigma\hookrightarrow Y$ and $\Sigma'\hookrightarrow Y'$ be embedded surfaces with induced open book foliations $\Fob=(E, \pit,H=H_+\cup H_-)$, $\Fob'=(E',\pit', H'=H'_+\cup H'_-)$. Suppose that there is a diffeomorphism $\psi\colon \Sigma\to \Sigma'$ that takes the two open book foliations to each other i.e., $\psi(E)=E'$, $\pit'\circ\psi=\widetilde{\pi}$ and $\psi(H_\pm)=H_\pm'$. Then there are neighbourhoods $N=N(\Sigma)$ and $N'=N(\Sigma')$ and an extension of $\psi$ to $\Psi\colon N\to N'$ so that 
\begin{enumerate}
\item $\Psi(B)=B'$
 \item $\pi=\pi'\circ\Psi$;
 \item $\Psi(B\cap N)=B'\cap N'$ and the trivialisation of $N(B)\cap N\cong (B\cap N)\times D^2$ in which $\pi=\vartheta$ maps to the trivialisation of $N(B')\cap N'\cong (B'\cap N')\times D^2$ in which $\pi'=\vartheta$. %
 \end{enumerate}
Moreover one can choose supported contact structures $(M,\xi)$ and $(M',\xi')$ for $(B,\pi)$ and $(B',\pi')$,  respectively, so that $\Psi$ is a contactomorphism between $(N,\xi\vert_{N})$ and $(N',\xi'\vert_{N'})$. 
\end{proposition}
\begin{proof}
Let us first describe local models around the points of $\Sigma\subset Y$. For each point $p\in {\Sigma}$ we will give a neighbourhood $D_p^2\times I$ of $p$ in $Y$ with coordinates adapted to $(B,\pi)$. These coordinates are chosen by a repeated use of the implicit function theorem, and both the neighbourhood $D_p^2$ and the interval $I$ might shrink as we make our additional choices. 

In the neighbourhood of a \emph{regular point} $p$ of the foliation ${\F}_{ob}$ we can choose local coordinates $(u,v,z)$ on $Y$ so that $v=\pi-\pit(p)$, ${\Sigma}=\{z=0\}$ with orientation $(\partial u,\partial v)$, coorientation $\partial z$ and the foliation ${\F}_{ob}$ is directed by $\partial u$. We call such a coordinate system in neighbourhood that only contains regular points of ${\F}_{ob}$ an \emph{adapted coordinate system}. The set of adapted coordinates in a given neighbourhood $U$ is convex.

Around an \emph{elliptic point} $e_\pm$ of ${\F}_{ob}$, we know that $B\pitchfork {\Sigma}$ at $e_\pm$, and $N(B)\cong B(\varphi)\times D^2(r,\vartheta)$. In these coordinates $e_\pm=(\varphi_0,0,0)$, and in a sufficiently small neighbourhood we can write $\Sigma\cap N(B)$ as the graph of a function $f\colon \{\varphi_0\}\times D^2\to \R$ that fixes $\{\psi_0\}\times\{0\}$. Since $\Sigma$ is transversal to $B$ we have $df\neq d\varphi$ at the origin of $D^2$ $\times \varphi_0$, so we can use the implicit function theorem to choose coordinates $(z=f-\varphi$, $r,\vartheta)$. In these coordinates $\Sigma=\{z=0\}$, $B$ is oriented by $\partial z$, $\Sigma$ is cooriented by $\pm\partial z$ and $\pi=\vartheta$.

%\jel{This seems better. Erase previous paragraph?} \vv{As I got confused with it I added the proof, we might remove it in a  later phase, but for now I want it to stay.}
%Choose a trivialisation of $N(B)\cong B(\varphi)\times D^2(r,\vartheta)$ so that $\Sigma=\{\varphi=0\}$ and $\pi=\pit$. 

%with $\pi=\vartheta$ and $e_\pm=(0,0,0)$. 
%We choose local coordinates, where ${\Sigma}=\{\varphi=0\}$, and the orientation of ${\Sigma}$  (away from $e_\pm$) is given by $(\pm \partial r,\partial \vartheta)$ and ${\F}_{ob}$ is directed by $\pm \partial r$ . The binding $B$ is oriented by $\partial \varphi$.

In the neighbourhood of a hyperbolic point $h_\pm$  the function $\pi\vert_{{\Sigma}}$ is Morse  with $h_\pm$  an index 1 critical point. By the Morse Lemma and since the differential of $\pi$ in the $I$-direction is nonzero, we can use the implicit function theorem and choose coordinates $(x,y,z)$ so that ${\Sigma}=\{z=0\}$ and $\pi-\pi(h_\pm)=z-y^2+x^2$. The surface ${\Sigma}$ is cooriented by $\pm\partial z$ and ${\F}_{ob}$ is directed by $y\partial x + x\partial y$.

As a next step we consider the intersections of these coordinate systems.  First, by choosing sufficiently small neighbourhoods we can  ensure that the neighbourhoods of ellliptic and hyperbolic points described above are all disjoint. 

If $q$ is a regular point that is in the neighbourhood of another regular point $p$ with a coordinate system $(u,v,z)$ as above, then we can write $q=(u_0,v_0,z_0)$, and construct a new adapted coordinate system: \[(u',v',z')=(u-u_0,v-v_0,z-z_0).\]
 
Let $p=(z_0, r_0,\vartheta_0)\neq (0,0,0)$ be a point in the neighbourhood of $e_\pm$. Then $\pi(p)=\vartheta_0$ and the coordinates:
\[(u',v',z')=(\pm (r-r_0),\vartheta-\vartheta_0,z-z_0)\] give an adapted coordinate system around $p$.

Similarly, let $p=(x_0,y_0,z_0)\neq (0,0,0)$ be a point on ${\Sigma}$ in the neighbourhood of $h_\pm$. 
Note that since we are on ${\Sigma}=\{z=0\}$ but in the complement of $(0,0,0)$, at least one of $x_0$ or $y_0$ must be nonzero. Without loss of generality we can assume that  $x_0>0$. In this case the coordinates 
\[(u',v',z')=(xy-x_0y_0,(z-x^2+y^2)-(z_0-x_0^2+y_0^2),(\log(x)+2z)-(\log(x_0)-2z_0))\] 
are defined in a neighbourhood of $x_0$ with $x>0$, and this gives an adapted coordinate system in a neighbourhood of $p$.

Finally, using these local models for $\Fob$ and $\Fob'$ we can define local maps that take the corresponding coordinate systems to each other. Then we can use a partition of unity to construct a global map $\Psi\colon N \to N'$ from the local ones. Near the elliptic points, the map brings the coordinate systems for the elliptic points to each other, so $\psi$ satisfies conclusion (3). Conclusion (1) is automatically satisfied by the construction. As for conclusion (2), we need to check that $\pi'\circ \psi=\pi$. This is certainly true for the local maps, and the construction of $\psi$ used their convex combinations. In the above change of coordinate systems, the value of $\pi$ was implicit in the system, so we can assume that we only need to take the convex combination of adapted coordinates in the neighbourhood of regular points. These form a convex set, thus the value of $\psi\circ \pi$ is unchanged while taking their convex combination.

As for the second part, concerning compatible contact structures, let $(S,h)$ be an abstract open book corresponding to $(B,\pi)$. From now on we will assume that $M$ is identified with $M_{(S,h)}$. We briefly recall the Thurston--Winkelnkemper construction \cite{TW} of a contact structure $\widetilde{\xi}=\ker\widetilde{\alpha}$ on $M$ supported by $(B,\pi)$. The construction depends on 
a 1-parameter family of 1-forms $(\beta_t)_{t\in [0,1]}$ on the page $S$, such that $d\beta_t$ is an area form on $S$ with total area $2\pi$ and $h_*\beta_0=\beta_1$, and a sufficiently large constant $\widetilde{C}$. Then the contact form $\widetilde{\alpha}$ is defined away from $N(B)$ by $\beta_t+\widetilde{C}dt$. In a smaller neighbourhood of the binding identified as $B(\varphi) \times D^2(r,\vartheta)$, the contact form $\widetilde{\alpha}$ is given by $2d\varphi+r^2d\vartheta$. In the complement of the two neighborhoods the construction gives an explicit extension of the two 1-forms. 

Let $(S',h')$ be the abstract open book corresponding to $(B',\pi')$, and as before assume that $M'$ is identified with $M_{(S',h')}$. Take the 1-parameter family of 1-forms  $\widetilde{\beta}'_t=(\Psi\vert_{(S\times\{t\})\cap U})_*\beta_t$ on $(S'\times \{t\})\cap U'$ and choose an area form on $S'$ so that $d\widetilde{\beta}'_t$ has total area less than $2\pi-\varepsilon$ on any closed subset of $U'$.
Since $\Psi$ respects the monodromies $h$ and $h'$, we have that 
$\widetilde{\beta}_1=h'_*\widetilde{\beta}'_0$ wherever both are defined. Thus we can extend $\widetilde{\beta}'_t$ to an area form $\beta'_t$ on $S'_t$ satisfying the conditions of the Thurston and Winkelnkemper construction, and now a compatible contact form may be defined by a choice of a sufficiently large constant $\widetilde{C}'$. 

Let $C=\max\{\widetilde{C},\widetilde{C}'\}$ and define the contact forms $\alpha$ on $M$ and $\alpha'$ on $M'$ by the Thurston--Winkelnkemper construction using the parameters $\beta_t$ and $C$, and $\beta_t'$ and $C$, respectively. For the corresponding contact structures $\xi=\ker\alpha$ and $\xi'=\ker\alpha'$ we get that $\Psi\vert_N$ is a contactomorphism between $(N,\xi\vert_N)$ and $(N',\xi'\vert_{N'})$, as needed.
\end{proof}
In order to give an explicit model for the open book in $N(\Sigma)$, in the next subsection we construct a simple open book for $\Sigma\times S^1$ with a prescribed open book foliation on $\Sigma\times \{0\}$.

\marginpar{\vv{LF part -- stop}}

\subsection{An open book for a surface bundle with prescribed open book foliation}\label{sec:egcircle}  \marginpar{\jel{LF}}
In this section we will show that every foliation that ``looks like''  an open book foliation is in fact an open book foliation. % \marginpar{\jel{I don't think I agree, as ob implies that the surface is embedded in a fibration.}\vv{Let's discuss!}}
Let $\Sigma$ be a surface and consider the tuple $\F=(E, \pit,H=H_+\cup H_-)$, where $E$ is a discrete set of points, $\pit\colon \Sigma\!\smallsetminus\! E\to S^1$ is an $S^1$-valued Morse function with only index 1 critical points $H$, and in a $D^2$ neighbourhood of each $e\in E$, $\pit$ restricts to $\pm \vartheta$ in polar coordinates $(r,\vartheta)$ on $D^2$. This local model separates the set of elliptic points $E$ as the union of two subsets $E_+$ and $E_-$. Note that the separation of $H$ into $H_+$ and $H_-$ is part of the defining data, rather than a consequence of $\pit$. The vector $\partial \pit$ coorients the leaves $\pit^{-1}(t)$ and, because $\Sigma$ is  oriented,   this orients the leaves as well. It is immediate that the foliation induced by  embedding  $\Sigma$ in an open book does have these properties. 

Use the given data to construct a dividing set $\Gamma=\partial N(G_{\scriptscriptstyle{++}})$ for the open book foliation, as described in Section~\ref{sec:charfol}.

In fact $\pit\vert_\Gamma$ is a covering of $S^1$ of degree $n$, where $n=|E_+|=|E_-|$. Let $\{\Gamma_i\}_{i=1}^k$ be the set of connected components of $\Gamma$ and let $n_i$ be the degree of $\pit\vert_{\Gamma_i}$. Note that $n=\sum_{i=1}^k n_i$. Then we can choose local coordinates $(v,u)$ on $A_i=N(\Gamma_i)$, so that $\pit=n_iv$, $\Gamma=\{u=0\}$ and $\partial u$ directs the level sets $\pit^{-1}(t)$. Let $A=\cup A_i=N(\Gamma)$, and $R_\pm'=R_\pm\!\smallsetminus\! A$. 
Next we construct a characteristic foliation on $\Sigma$ that is also divided by $\Gamma$:

\begin{lemma}[approximating $\F$ with characteristic foliations]\jel{moved to Chapter 3}%\label{lem:approx}
Let $\Gamma(\F)$ be the dividing curve and $R_\pm(\F)$ be the corresponding positive and negative regions of the open book foliation $\F=(E, \pit,H=H_+\cup H_-)$. 
Then there is a 1-form $\beta$ that agrees with $d\pit$ away from a small neighbourhood of the singular points, and $\pm d\beta>0$ on $E_\pm\cup H_\pm$,  so that the foliation $\F_\beta$ defined by $\beta$ has the same singular points, it is $\delta$-isotopic to $\F$, and $G_{\scriptscriptstyle{++}}(\F_\beta)\subset R_+(\F)$.

Moreover there is a positive function $g\colon \Sigma\to \R_{>0}$ so that $\beta'=g\beta$ is divided by $\Gamma$, (i.e., $\pm d\beta'>0$ on $R_\pm(\F)$ and $\beta\big(T\Gamma(\F)\big)>0$). Furthermore, we may assume that $g<1$ on $A=N\big(\Gamma(\F)\big)$. 
\end{lemma} 
\begin{proof}
For the first statement we start with the 1-form $d\pit$ on $\Sigma\!\smallsetminus\! E$ and modify it in the neighbourhood of the singular points of $\F$.

Recall that an elliptic point $e\in E_\pm$ has a neighbourhood $D^2_\varepsilon(r,\vartheta)$ where $\pit=\pm\vartheta$, so $d\pit=\pm 1$ on $D^2_\varepsilon \!\smallsetminus\!\{e\}$. Define $\beta=\pm\Psi^{\varepsilon}_{\varepsilon/2}r^2d\vartheta$, where $\Psi^{\varepsilon}_{\varepsilon/2}$ is a smooth bump function that is $1$ for $r<\varepsilon/2$, $0$ for $r>\varepsilon$ and strictly monotonically decreasing on $[\varepsilon/2,\varepsilon]$. At $e$ we have $\pm d\beta=2r dr\wedge d\vartheta$, which is a positive multiple of a volume form. 

In a neighbourhood of a  hyperbolic point $h\in H_\pm$, we can chose local coordinates  so that $\pit=x^2-y^2$. Thus $d\pit=2xdx-2ydy$ and $d^2\pit=0$.  Let $\beta=d\pit\pm \Psi^\varepsilon_{\varepsilon/2} xdy$. Then, as $d\Psi^\varepsilon_{\varepsilon/2}=0$ at $r=0$, we have that $\pm d_h\beta= dx\wedge dy$, a positive multiple of the volume form. 

Extend the 1-form on $\Sigma\setminus N(E\cup H)$ as $d\pit$ to  obtain a 1-form $\beta$ that satisfies the conditions of the first claim. 

Without the assumption $g<1$ on $A$, the second statement is standard in contact geometry. \marginpar{\vv{I found some sort of reference in John's notes on convex surfaces Thm 2.20, but there the statement is for $X$ and he changes $\omega$.. I will also check Giroux later.}} We will recall the proof in our context to see that we can prescribe $g$ to be arbitrarily small where required. Choose a Morse function $h$ on $\Sigma$ whose gradient flow with respect to some metric  directs $\F_\beta$ and satisfies the following conditions:
% \vv{such a Morse function has been used by Kyle as well, so maybe we don't need to prove its existence} \jel{Is this meant to be a globally defined function?  I think KH only constructs this on a subsurface where existence is clear.} \vv{Yes, this is global, the existence should be clear everywhere too, this is some sort of arclength of the leaves.. Kyle uses it in Example 4.3. He also gives a } 
\begin{itemize} 
\item[-] $\Gamma=h^{-1}(0)$;
\item[-] $A=h^{-1}[-\varepsilon,\varepsilon]$, so that $h=u$;
\item[-] $\partial v$ orients the level sets of $h$. 
\end{itemize}
Such a Morse function exists by Theorem B of \ref{Smale}, and we  use it to define
% https://web.ma.utexas.edu/users/dafr/M392C-2018-MorseTheory/Readings/Smale2.pdf  So we choose local Morse models near H and then Smale promises a global Morse function.  
 $g=h^2+1-2\varepsilon$.  Assuming that $\varepsilon<1/2$, the function $g$ is indeed positive on $\Sigma$, $\beta'(T\Gamma)=g\beta(\partial v)=g\d\pit(\partial v)>0$, and 
\[\pm d\beta'=\pm dg\wedge\beta\pm gd\beta.\]
The second term  on the right vanishes away the singular points and is a positive multiple of a volume form near the singular points. As for the first term, we have $dg=2hdh$.  Recall that the gradient vector field of $h$ directs $\F_\beta$, so $dh\wedge\beta>0$ and the sign of $h$ is $\pm$ in $R_\pm$. 
This proves that $\pm d\beta'>0$ everywhere on $R_\pm$ and as required, $g=h^2+1-2\varepsilon\le 1-\varepsilon<1$ on $A$. 
\end{proof}

\begin{proposition}[Giroux, \cite{Gi}]%\label{prop:Gi} 
% Sivek Thm 21
\jel{moved to Chapter 3}
Suppose that $\beta'$ is divided by some dividing curve $\Gamma$, then there is a function $f\colon \Sigma\to [-1,1]$ such that $f^{-1}(\pm 1)=R_\pm'$; on $A$, $f$ depends only on $u$ and it is a monotonically decreasing function of $u$; and $f^{-1}(0)=\Gamma$ and $\alpha=\beta'+fd z$ is a contact form on $\Sigma\times I$. \marginpar{\vv{We should probably be able to give an explicit formula for $f$ using coordinates in $A$. That might be useful, otherwise it could depend on $\beta'$}}\qed
\end{proposition}

We use the functions $f$ form Proposition \ref{prop:Gi} and $g$ from Lemma \ref{lem:approx} to construct both a contact structure and an open book for a $\Sigma$-bundle over  $S^1$. Consider the product $\Sigma\times \R$ with the contact structure defined as the kernel of the 1-form \[\alpha'=\beta'+f dz.\] Let $B'=E\times \R$, where the orientation of $\{e\}\times \R$ is given by $\pm\partial z$ for $e\in E_\pm$. Consider the function \[\pi'=\pit+fz\colon \Sigma\times \R\to S^1,\] %here the sign ``$+$'' stands for the action of $\R$ by translation on $S^1=\R/\mathbb{Z}$. 
where adding $f(x,z)z\in \mathbb{R}$ to $\pit(x,z)$ indicates translation by the image of $fz$ in the quotient $S^1=\mathbb{R}\slash \mathbb{Z}$. 

We would like to glue $\Sigma\times \{0\}$ to $\Sigma\times\{l\}$ for some $l\in\mathbb{N}$ to get an open book and a contact structure for a $\Sigma$-bundle over  $S^1$ . As $f=\pm 1$ on $R_\pm'$ we have $\pi'(x,0)=\pi'(x,l)$ on $R_\pm'$. 
On $A_i=N(\Gamma_i)\cong\Gamma_i\times [-\varepsilon,\varepsilon]$, with coordinates $(v,u)$ chosen as in Lemma \ref{lem:approx}, we have $\pi'((v,u),l)-\pi'((v,u),0)=lf(v,u)$, where $f(v,u)$ is independent of $v$ %=\pit/n_i$ \jel{($\pit=n_i v$, but this is $n:1$ and not invertible.)} 
and monotonically decreases from $1$ to $-1$ in $u$. %along each level set $\pit^{-1}(t)$. 
This means that each level set of $\pi'\vert_{\Sigma\times\{l\}}$ restricted to $A_i$ consists of $n_i$ parallel curves connecting the points $(v,-\varepsilon)$ with $(v+2l/n_i,\varepsilon)$. %, here $u$ parametrises the components $\Gamma_i\cong\R/n_i\mathbb{Z}$ of $\Gamma$. 
When $2l$ is divisible by $n_i$, the endpoints of each component therefore have the same $v$ coordinate, as $v$ parmeterizes $S^1\cong \R/\mathbb{Z}$, and in fact, the curve intersects an arbitrary  $v=c$ segment $\frac{2l}{n_i}\in \mathbb{Z}$ times. 

Set  $l=\lcm\{n_i\}_{i=1}^k$ and consider the mapping torus $M_h(\Sigma)=\Sigma\times [0,l]/(x,0)\sim (h(x),l)$ \marginpar{\vv{we have 2 more $h$'s in the proofs earlier, as the function that defines $g$, and the generic hyperbolic points are also $h$'s. I think it's OK, but not ideal..}}
of the  diffeomorphism  \[h=\prod_{i=1}^k D_{\Gamma_i}^{\frac{2l}{n_i}},\] where $D_{\Gamma_i}^{n_i}$ is the right handed Dehn twist along  $\Gamma_i$. Then $\pi'(x,0)=\pi'(h(x),l)$ on $S^1$ and $\pi'$ descends as $\pi$ to  $M_h(\Sigma)\!\smallsetminus\! B$, where $B=B'\slash\sim$. 

Notice, too, that since $f$ depends only on $u$ and the Dehn twists were along the $v$-direction in the $A_i$, the 1-form $\alpha'$ descends  to $M_h$ as a 1--form $\alpha$, giving a contact structure $\xi$ on $M_h$. 

%what if \Gamma is only isotopic through curve transverse to $\F$

\begin{proposition}[Open book for $(M_h,\xi)$]\label{prop:obcyl} Via the construction above, any $\F$ determines an open book decomposition $(B,\pi)$ for $M_h$. Moreover, it supports the contact structure $\xi=\ker\alpha$. %defined as the kernel of $\alpha=g\beta+fdz$
\end{proposition} 
Before proving the above proposition, we reformulate what it means for an open book decomposition to support a contact form. 

\begin{lemma}\label{lem:ob} Let $B$ be a (positive) transverse  knot in $(M,\xi=\ker\alpha)$ and suppose the map $\pi\colon M\!\smallsetminus\! B\to S^1$  restricts as $\pi=\vartheta$ in a neighbourhood $N(B)=B\times D^2(r,\vartheta)$ of $B$. Then the pair $(B,\pi)$ is an open book  supporting the contact form $\alpha$ if and only is $d\pi\wedge d\alpha>0$. \qed
\end{lemma}

%\begin{proof} \vv{As the proof is trivial, I am not sure we should keep it at the end.}\jel{ agreed }
%With the assumption near $B$, the statements $(B,\pi)$ being an open book decomposition and $d\pi\neq 0$ are equivalent, and $d\pi\neq 0$ also follows from $d\pi\wedge d\alpha>0$, thus in the following we can assume that $d\pi\neq 0$. This means, that we can choose a local coordinate system $(u,v,w)$ so that $\pi=u$ and the level sets of $\pi$ are parametrised by $(v,w)$. By definition we can compute $d\pi\wedge d\alpha(\partial u,\partial v,\partial w)$ as 
%\[d\pi(\partial u)d\alpha(\partial v,\partial w)+d\pi(\partial v)d\alpha(\partial w,\partial u)+d\pi(\partial w)d\alpha(\partial u,\partial v).\]
%As $d\pi=du$, we have:
%\begin{equation*}\label{eq:1}(d\pi\wedge d\alpha)(\partial u,\partial v,\partial w)=d\alpha(\partial v,\partial w)\end{equation*}
%And the left hand side being positive is equivalent to $d\alpha$ being an area form on the level sets of $\pi$, while the right hand side being positive is equivalent to $d\pi\wedge d\alpha$ being a volume form. Thus the above equation proves the statement. 
%
%Which means that $d\alpha$ is an area form on the level sets of $\pi$.
%
%If on the other hand $\alpha$ is supported by $(B,\pi)$, then by definition $d\pi\neq 0$, and we can use the same local coordinates as before, and we again get
%\[(d\pi\wedge d\alpha)(\partial u,\partial v,\partial w)=d\alpha(\partial v,\partial w)>0\]
%This time we deduce that the right hand side is a volume form on $Y$. So the equivalence is proved.  
%\end{proof}

\begin{proof}[Proof of Proposition \ref{prop:obcyl}.]

In a neighbourhood of $B$ the function $\pi$ restricts as $\pm(\vartheta+z)$,
 so we see that $\pi^{-1}(t)$ indeed enters $N(B)$ as a Seifert surface. If we evaluate $\alpha$ on $TB=\pm\partial z$ we get $\alpha(\pm\partial z)=1>0$, as needed. 
 
For the second step,  by Lemma \ref{lem:ob} it is sufficient to show that $d\pi\wedge d\alpha >0$ on $M_h\!\smallsetminus\! B$. Since $\alpha$ is a contact form,  $\alpha\wedge d\alpha>0$, yielding the following:
\[
(\beta'+fdz)\wedge (d\beta'+df\wedge dz)=dz\wedge(\beta'\wedge df+fd\beta')>0.
\]
%\textcolor{green}{\[(g\beta+fdz)\wedge (dg\wedge \beta +gd\beta+df\wedge dz)=dz\wedge(g\beta\wedge df+fdg\wedge\beta+fg d\beta)>0.=\]}
This in turn is equivalent to the condition that 
%\textcolor{green}{\begin{equation*}\label{eq:area} \omega_0=g\beta\wedge df+fdg\wedge\beta+fgd\beta\end{equation*}}
\[
\omega_0=\beta'\wedge df+fd\beta'
\]
 is an area form on $\Sigma$. 

We compute $d\pi \wedge d\alpha$:
%\textcolor{green}{\[(d\pit+zdf+fdz)\wedge(dg\wedge\beta+ gd\beta+df\wedge dz)=dz\wedge(d\pit\wedge df+fdg\wedge\beta+fgd\beta)
%\]}
\[
(d\pit+zdf+fdz)\wedge(d\beta'+df\wedge dz)=dz\wedge(d\pit\wedge df+fd\beta')
\]
Thus we require that %\textcolor{green}{$\omega'=d\pit\wedge df+fdg\wedge\beta+fgd\beta$}
 $\omega'=d\pit\wedge df+fd\beta'$ is an area form on $\Sigma$.  To check this, we compare the given form to the area form $\omega_0$ given by the contact condition and substitute $\beta'=g\beta$:
\[\omega'=\omega_0+(d\pit-g\beta)\wedge df.\]
In the following we will prove that $(d\pit-g\beta)\wedge df\ge 0$, which implies that  $\omega'>0$.
%The difference between the restrictions of $\alpha'\wedge d\alpha$ and $d\pi\wedge d\alpha$ to $T\Sigma$ is:
%\[(d\pit-g\beta)\wedge df\]

On $R_\pm'$ the differential $df$ is 0, thus $\omega'=\omega_0$, so it is indeed an area form.

%\jel{Away from $H$, we use the parameterization of $\Sigma$ by $(u,v)$ and recall that  $\beta=d\pit$.  We must show that  that \[d\pit\wedge df+fdg\wedge\beta+fgd\beta=d\pit\wedge df+fdg\wedge d\pit= (f dg -df)\wedge d\pit\] is an area form.  From \ref{eq:area} we have that \[gd\pit\wedge df+fdg\wedge d\pit=(f dg - g df )\wedge d \pit=k' du \wedge dv\] for some positive function $k'$.  Since $d\pit$ is a positive scaling  of $dv$, we can interpret this as $f dg -g df=k du$ for some positive function $k$.  By hypothesis, $g>0$ and $-df (\partial u)>0$, \marginpar{\jel{Away from $A$, the claim  $-df (\partial u)>0$ needs to be justified.}} so the second summand is positive.  If $g\leq1$, then it follows that $f dg-df$ is also a positive multiple of $du$, and is therefore an area form as desired.  }
On $A$,  $\beta=d\pit$, so we have   
\[(d\pit-g\beta)\wedge df=(1-g)d\pit \wedge df.\]
Recall that on $A$, $f$ depends only on $u$ and is decreasing, while %decreases in $u$ while 
$\pit$ depends only on $v$ and is increasing. %increases in it.  
Thus $d\pit \wedge df$ is an area form, and as $g>1$ on $A$, so is $(1-g)d\pit \wedge df$, as desired. 
\end{proof}

Note that the pages of $(B,\pi)$ are $l$-fold covers of $\Sigma\!\smallsetminus\! E$ via the map from $\pi^{-1}(t) \to \Sigma\!\smallsetminus\! E$ defined by  $(x,z)\mapsto x$. 

Recall that Corollary~\ref{cor:lm} proposes an explicit local model for the open book in the neighbourhood of $\Sigma$ with a given open book foliation. We prove this next.

\jel{Corollary has been moved earlier, but perhaps restate here?}

Notice that in this local model, the induced open book foliations on the nearby surfaces $\Sigma\times\{z\}$ are topologically conjugate and \vv{$\delta$ isotopic} to $\F$. One can also understand the restrictions of a page $\pi^{-1}(t)$ onto $N(\Sigma)$; they are $\pit^{-1}[t-\eta,t+\eta]\cap R_+'$ and $-\left(\pit^{-1}[t-\eta,t+\eta]\cap R_-'\right)$ glued together with a twisted band. If the interval $ [t-\eta,t+\eta]$ contains only regular values of $\pit$, then $\pi^{-1}(t)\cap N(\Sigma)$ is just a union of $|E_+|=|E_-|$ strips; these are rectangles embedded into $N(\Sigma)$, so that a pair of its opposite sides are embedded into $\Sigma\times\{-\eta\}$ and $\Sigma\times \{\eta\}$. If $[t-\eta,t+\eta]$ contains a singular value, then one component of  $\pi^{-1}(t)\cap N(\Sigma)$ is a ``cross'', embedded as a saddle surface. See Figure \ref{} \marginpar{\vv{draw Figure}}. The intersection $\pi^{-1}(t)\cap N(\Sigma)$ is singular when $t\pm \eta$ is a singular value. 

\begin{figure}[h]
\begin{center}
\includegraphics[scale=0.3]{layer}
\caption{Level set near $A\times [-\eta,\eta]$}\label{fig:cobordism}
\end{center}
\end{figure}

\marginpar{redundant?  compare to para before Prop 3.4 and paras before 4.2.} From now on, we will use the term \emph{open book foliation} for any tuple $\F=(\pit,E,H=H_+\cup H_-)$ as above. Specifically,  we require only that $\pit$ is an $S^1$-valued Morse function with only index 1 critcal points at $H$ with distinct critical values  and prescribed local models $\pit=\pm \vartheta$ near the elliptic points, regardless of whether it is induced by an embedding into a classical open book or not.  The \emph{reparametriztaion} of the open book foliation $\F$  with the diffeomorphism $g\colon S^1\to S^1$ is the open book foliation $g(\F)=(\pit\circ g,E,H=H_+\cup H_-)$. Reparametrization of open book foliations defines an equivalence relation, and the equivalence class of the open book foliation $\F$ is denoted by $[\F]$.

\marginpar{\jel{LF stop}}

\subsubsection{Trivial foliated open book}
In the proof of the Expansion Theorem above, the focus was was on the complement of the neighborhood of $\Sigma$. We will later have use for the neighborhood itself, however, so we summarize its properties here.  

Following the language and notation of Proposition~\ref{prop:exp},  $N(\Sigma)=\Sigma\times [-\varepsilon, \varepsilon]$ has two boundary components printed with $\mathcal{F}_\pi$ and $-\mathcal{F}_\pi$, respectively.  A small perturbation of $\pi'$ may be applied so that paired critical points have distinct critical values, and we retain the same label for the perturbed funciton.  Then level sets of   $\pi'$ have two possible forms.  For most values of $t\in S^1,( \pi')^{-1}(t)$ is a product of an interval leaf of the original open book foliation with $[-\varepsilon, \varepsilon]$.  Associated to each original hyperbolic point is a $t$-interval separating its images in $\mathcal{F}_{\pi'}$ and $\mathcal{F}_{\pi'}$; each level set associated to a $t$-valued in this interval  is a thickened $X$:  a union of two such rectangle pages glued along a pair of boundary intervals.

We call a foliated open book of this form a \emph{trivial open book}, and we will make use of these  later on. \marginpar{\jel{note Morse vs emb?}}

%From now on, it makes sense to call any tuple $\F=(\pit,E,H=H_+\cup H_-)$ as above (i.e., $\pit$ is an $S^1$-valued Morse function with only index 1 critcal points at $H$ with distinct critical values,  and local models near the elliptic points, where $\pit$ is $\pm$ the angle) an \emph{open book foliation} on $\Sigma$, independently on whether it is induced by an auxiliary open book or not. \marginpar{\vv{Do you like this?}} The \emph{reparametriztaion} of the open book foliation $\F$  with the diffeomorphism $g\colon S^1\to S^1$ is the open book foliation $g(\F)=(\pit\circ g,E,H=H_+\cup H_-)$. Reparametrization of open book foliations form an equivalnce relation, and the equivalence class of the open book foliation $\F$ is denoted by $[\F]$.
